# Supplementary material for: Vibronic fine structure in the nitrogen 1s photoelectron spectra from Franck-Condon simulations II: Indoles
Source: arXiv:2307.01510 source file (2023-07-04)
Supplement: Supplementary file 1 [file si.pdf]

# Supplementary Material for “Vibronic fine structure in the nitrogen 1s photoelectron spectra from Franck-Condon simulations II: Indoles”

Minrui Wei,<sup>1</sup> Lu Zhang,<sup>1</sup> Guangjun Tian,<sup>2</sup> and Weijie Hua<sup>1,\*</sup>

<sup>1</sup>*MIIT Key Laboratory of Semiconductor Microstructure and Quantum Sensing,  
Department of Applied Physics, School of Science,*

*Nanjing University of Science and Technology, 210094 Nanjing, China*

<sup>2</sup>*Key Laboratory for Microstructural Material Physics of Hebei Province,  
School of Science, Yanshan University, 066004 Qinhuangdao, China*

(Dated: July 4, 2023)

## S1. Supplementary analyses for the theoretical spectrum of each molecule

Figures S1-S17 collect the vibrationally resolved N 1s XPS spectra of the individual molecules simulated by the Duschinsky rotation (DR) method at the B3LYP level. These are the same results as in the main text, but with more detailed analyses. For each molecule, analyses are presented on the atom-specific contributions, the main vibronic transitions (sticks”), the contributions of the different 0- $n$  transitions, and the active vibrational modes in the final state. Active modes were selected based on the following thresholds for the Franck-Condon factors:  $F \geq 0.02$  (indole, 3-methylindole, and 3-formylindole) or  $F \geq 0.04$  (the remaining molecules).

## S2. Visualization of the Duschinsky matrices of additional molecules

Figures S18-S20 show the Duschinsky matrices of 9 molecules (in addition to the 6 molecules in Fig. 6b of the main text) to compare the mode mixing effects for amine and imine nitrogens. Two molecules (3-methylindole and 3-formylindole; both contain only amine nitrogens) were not analyzed.

---

\* wjhua@njjust.edu.cn

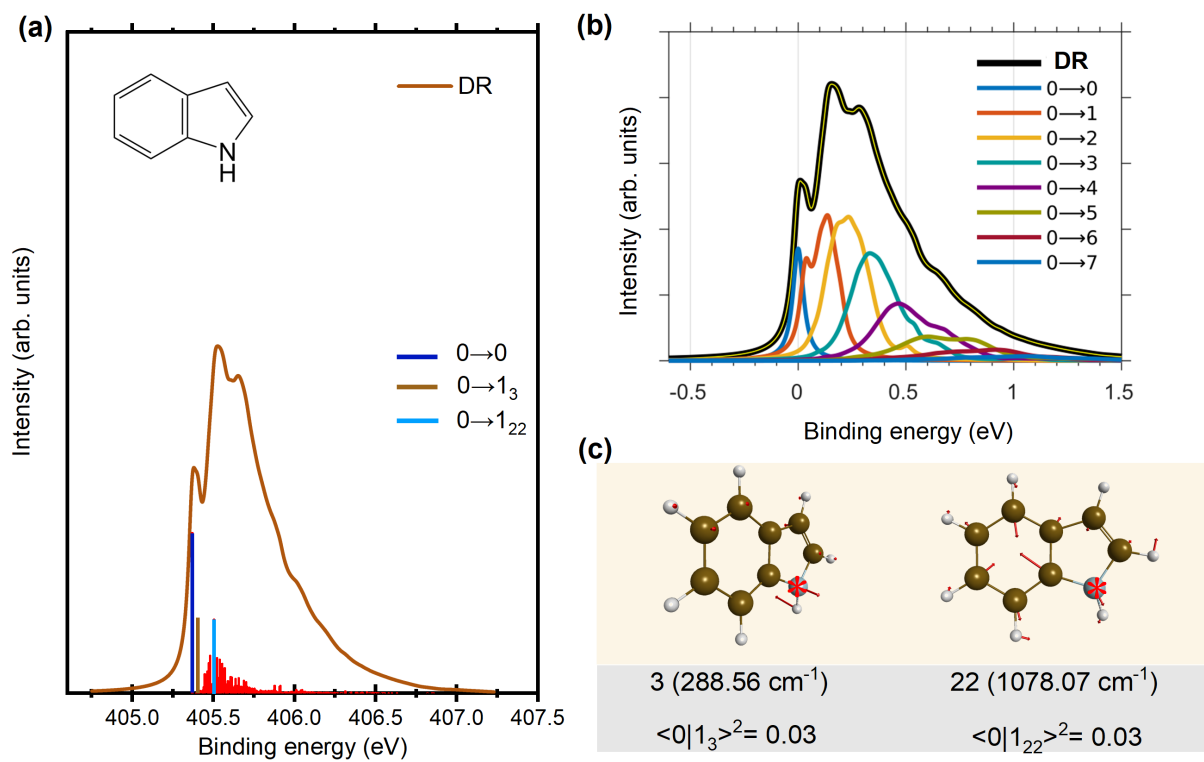

FIG. S1: (a) Simulated vibrationaly-resolved N 1s XPS spectrum of indole. (b) Analyses of contributions of different 0- $n$  transitions until convergence. 0-0 transition energy is taken as zero. (c) Active vibrational modes interpreted at the final state structure (**min FCH**). The core hole is indicated by an asterisk.

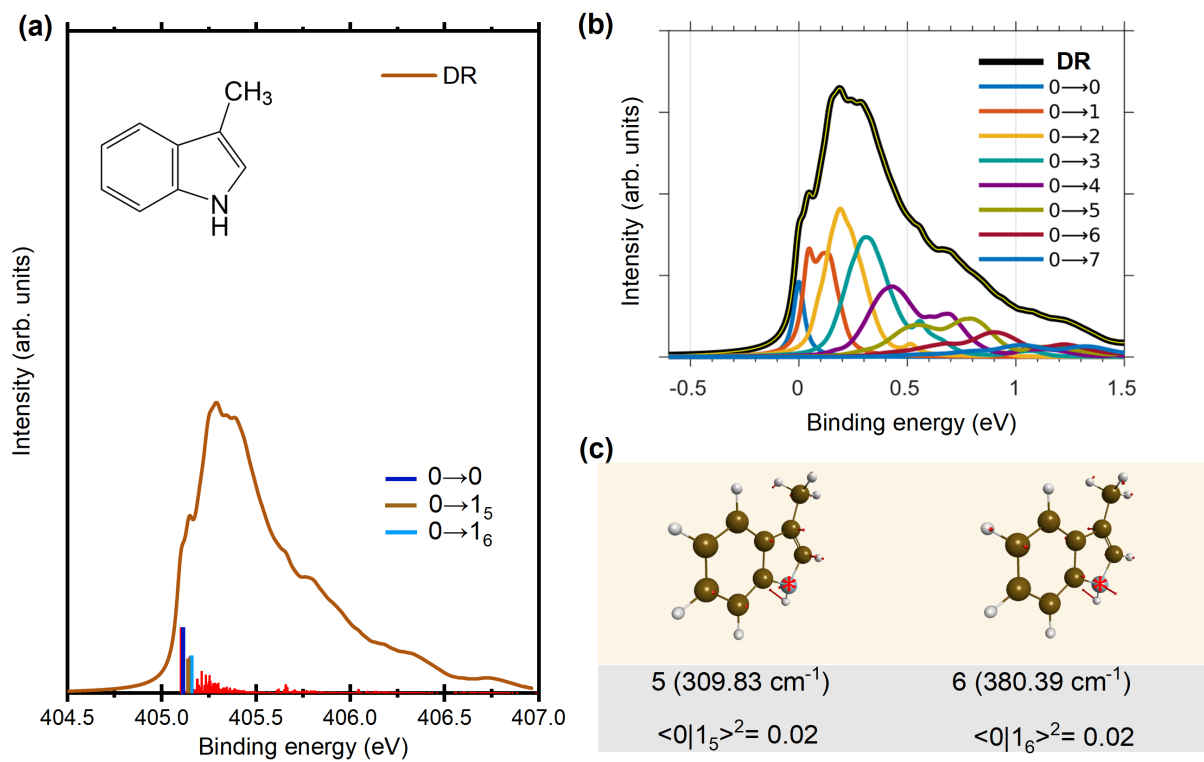

FIG. S2: The same as Fig. S1 for 3-methylindole.

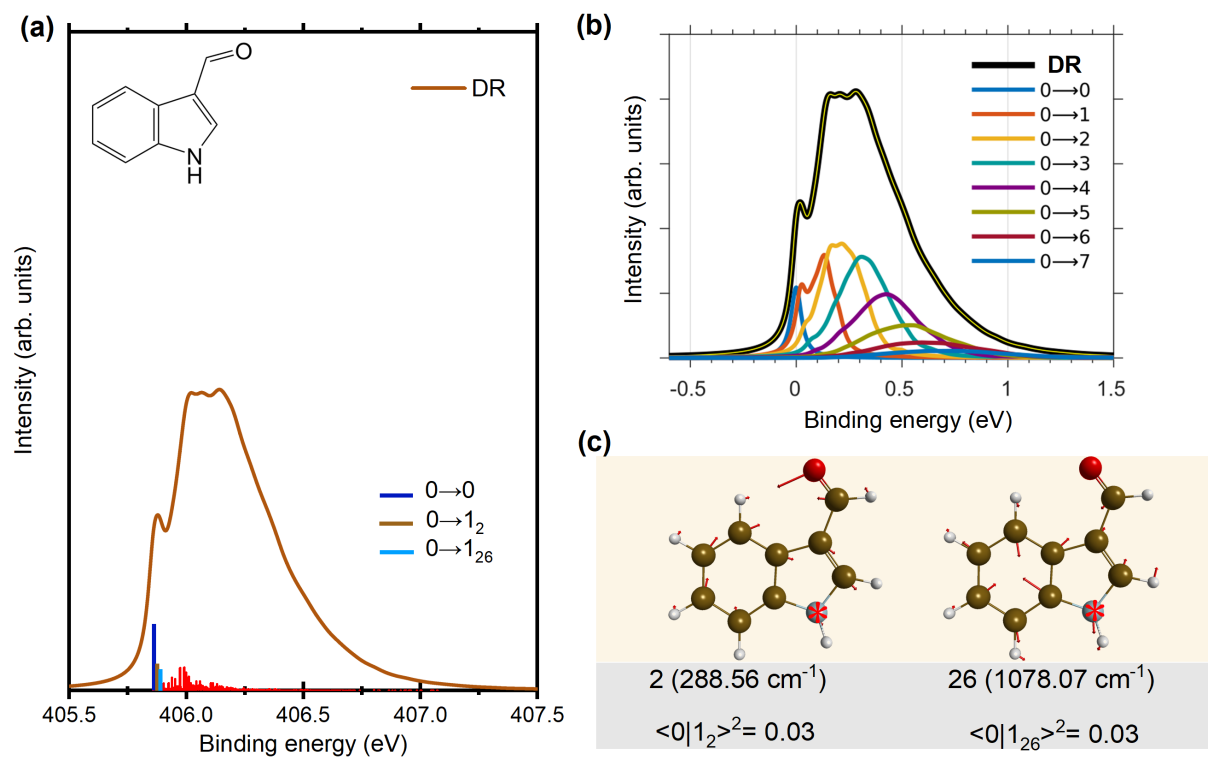

FIG. S3: The same as Fig. S1 for 3-formylindole.

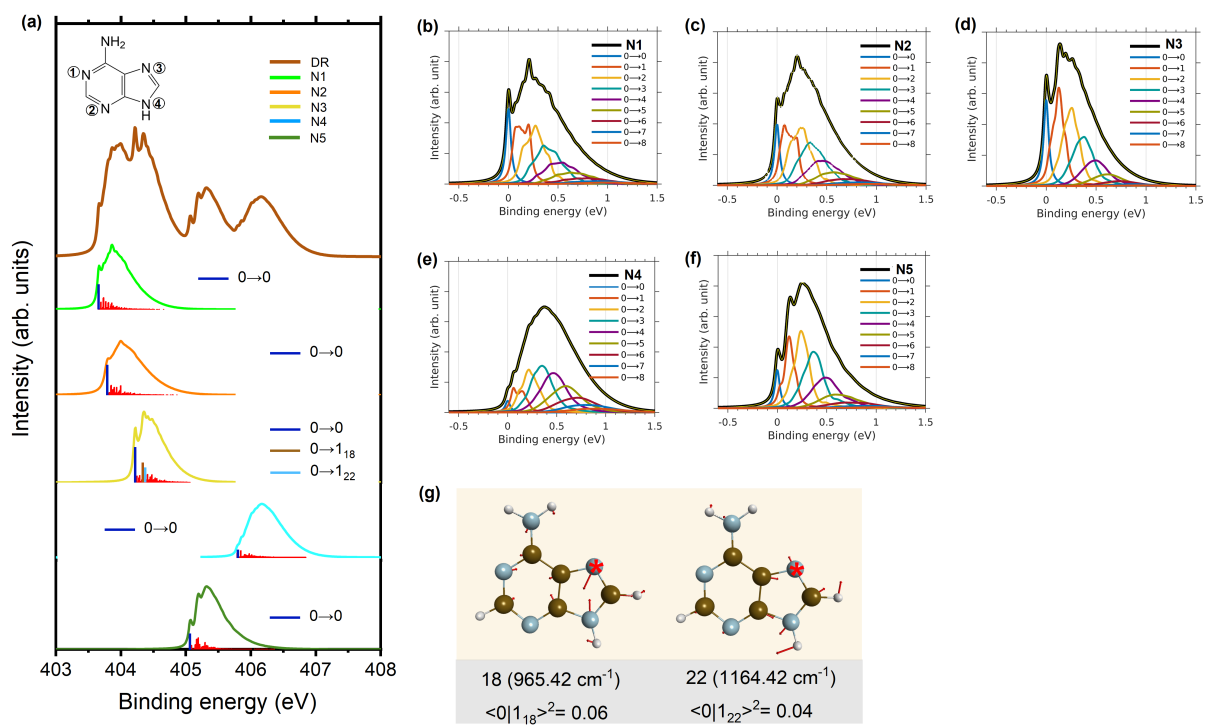

FIG. S4: (a) Simulated vibrationaly-resolved N 1s XPS spectrum of adenine. Atomic-specific contributions are given below the total spectrum. (b-f) The contribution of the different  $0 \rightarrow n$  transitions (until convergence) of N1-N5.  $0 \rightarrow 0$  transition energy is taken as zero. (g) Active vibrational modes interpreted at the final state structure (**min FCH**). The core hole is indicated by an asterisk.

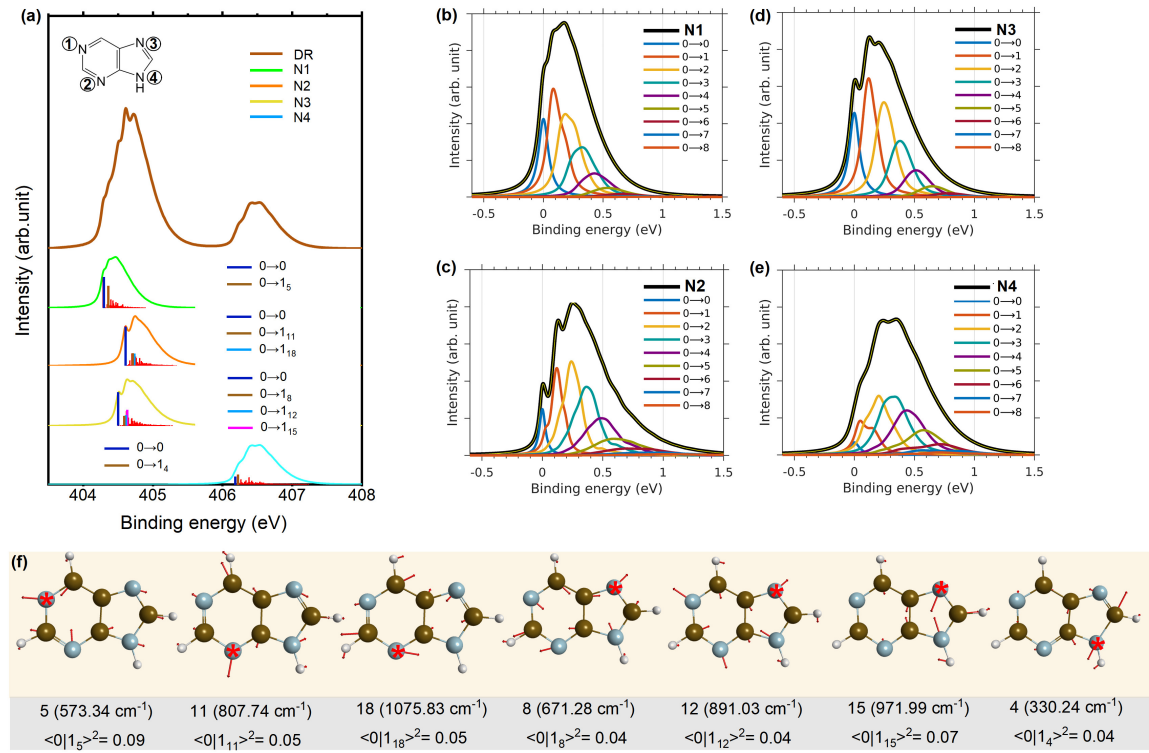

FIG. S5: (a) Simulated vibrationally-resolved N 1s XPS of purine. (b-e) The contribution of the different 0- $n$  transitions (until convergence) of N1-N4. 0-0 transition energy is taken as zero. (f) Active vibrational modes interpreted at the final state structure (**min FCH**). The core hole is indicated by an asterisk.

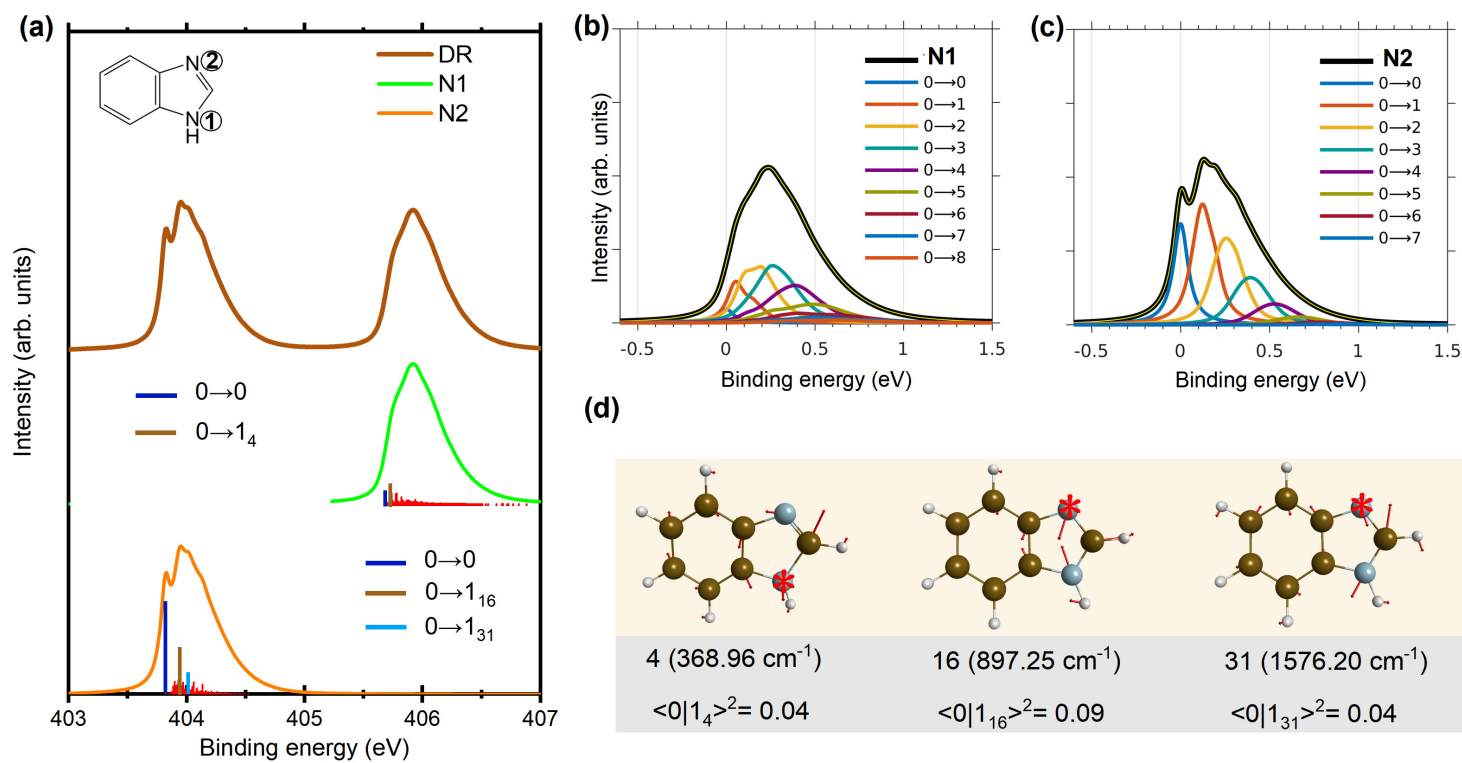

FIG. S6: (a) Simulated vibrationally-resolved N 1s XPS of benzimidazole. (b-c) The contribution of the different 0→n transitions (until convergence) of N1 and N2. 0→0 transition energy is taken as zero. (d) Active vibrational modes interpreted at the final state structure (**min FCH**). The core hole is indicated by an asterisk.

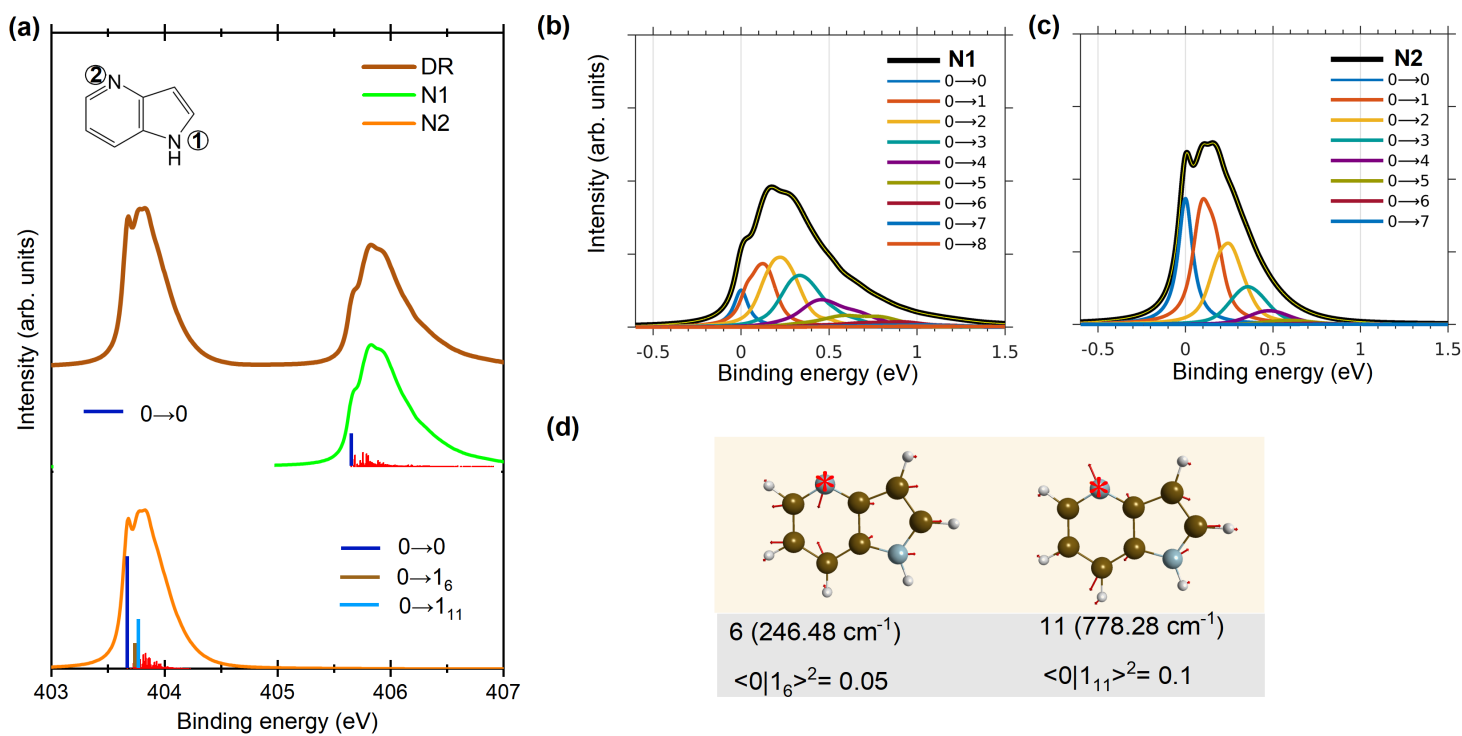

FIG. S7: The same as Fig. S6 for 4-azaindole.

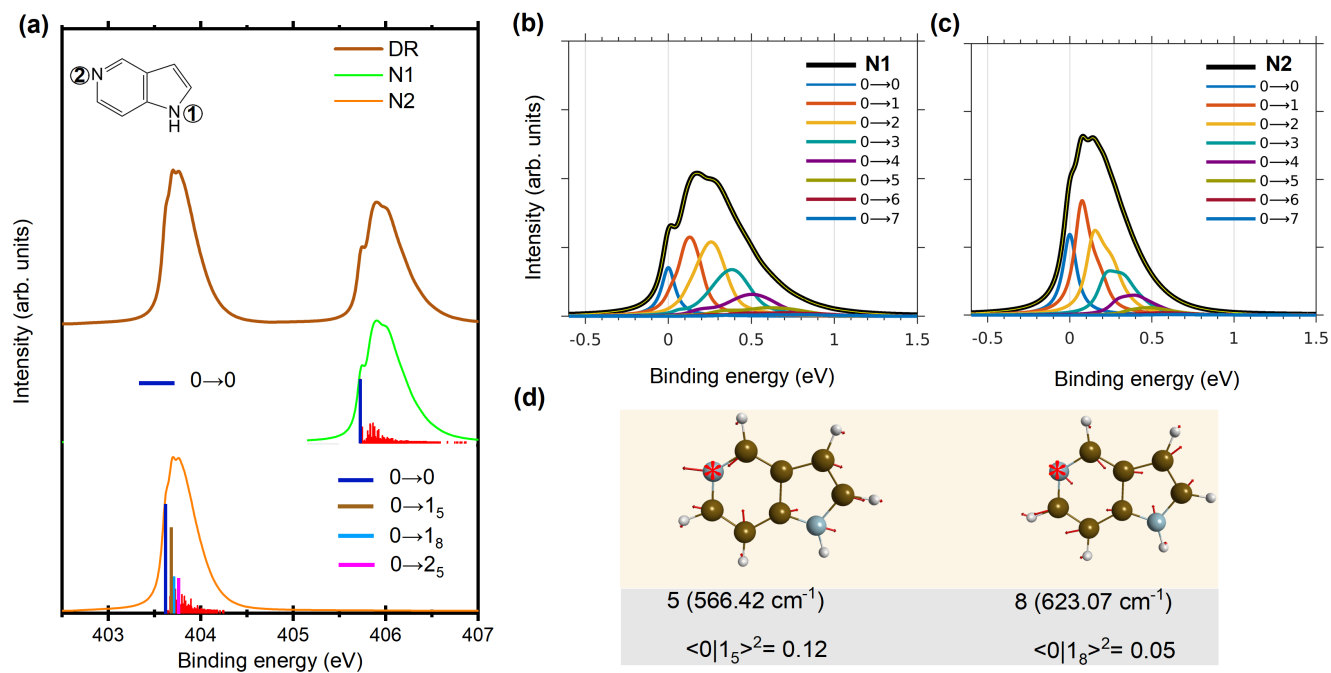

FIG. S8: The same as Fig. S6 for 5-azaindole.

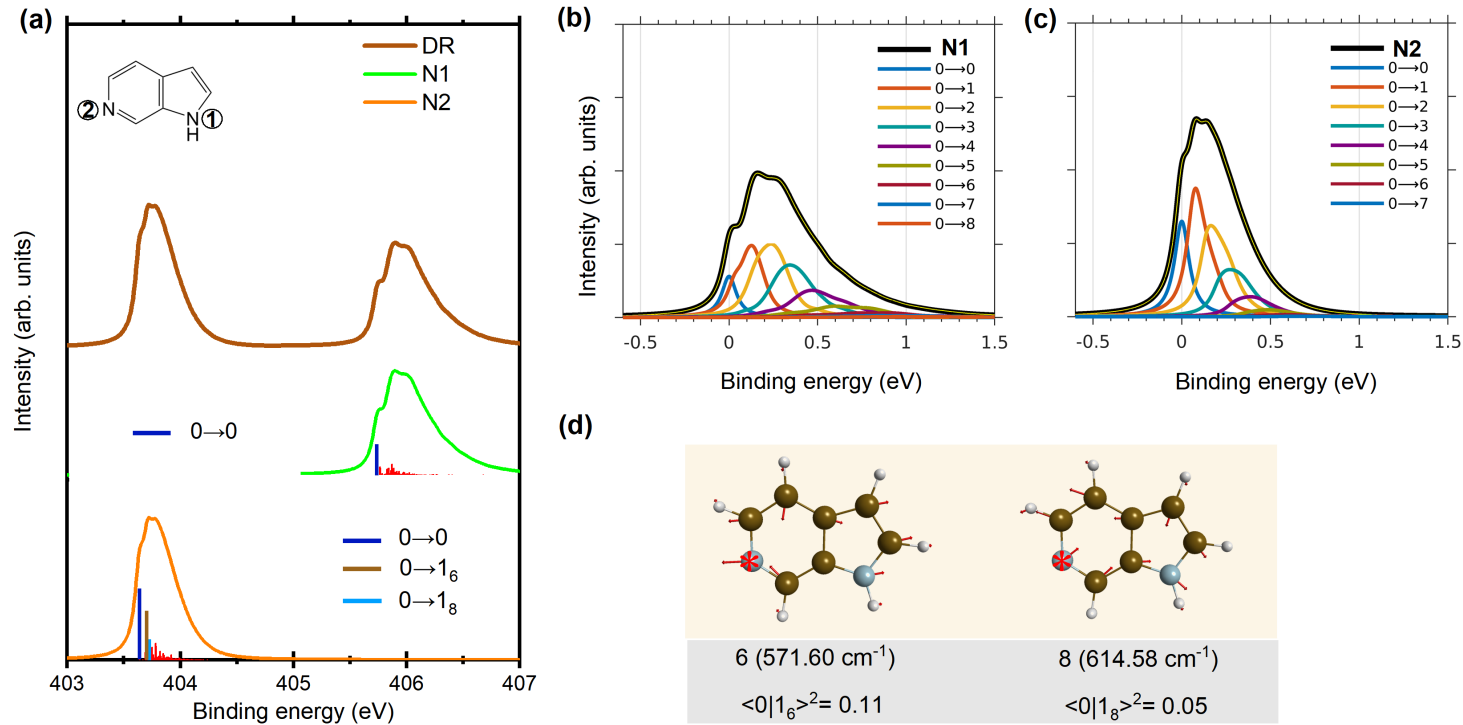

FIG. S9: The same as Fig. S6 for 6-azaindole.

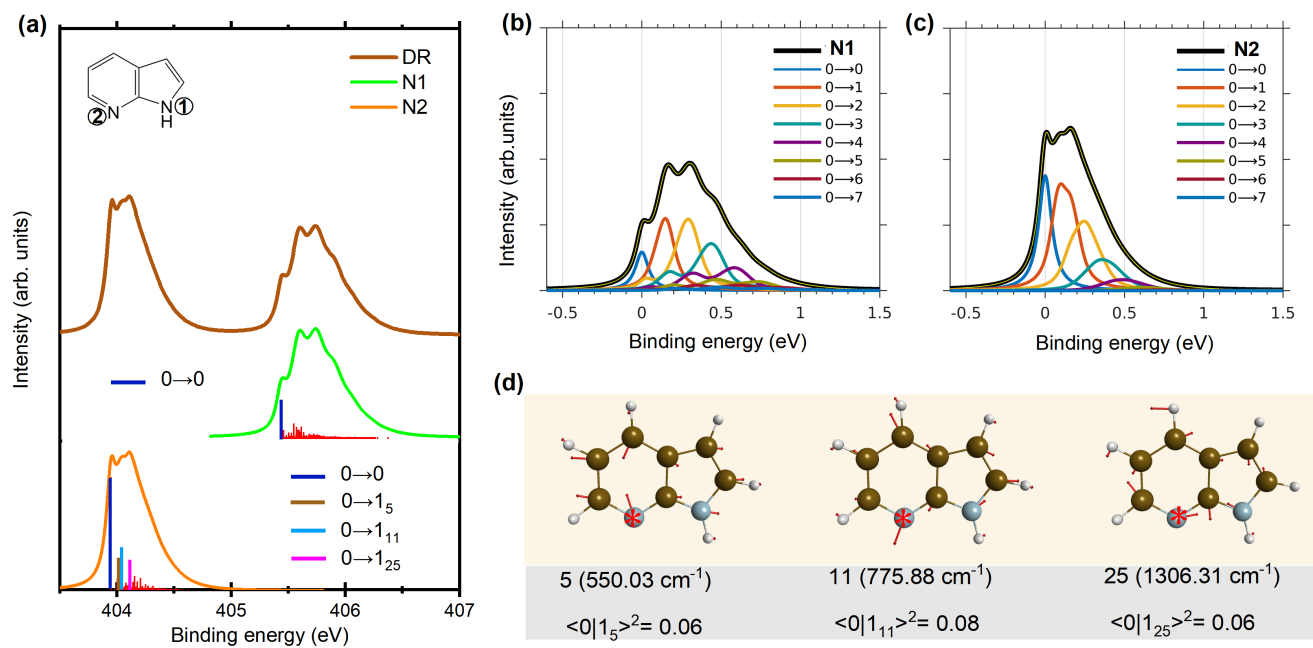

FIG. S10: The same as Fig. S6 for 7-azaindole.

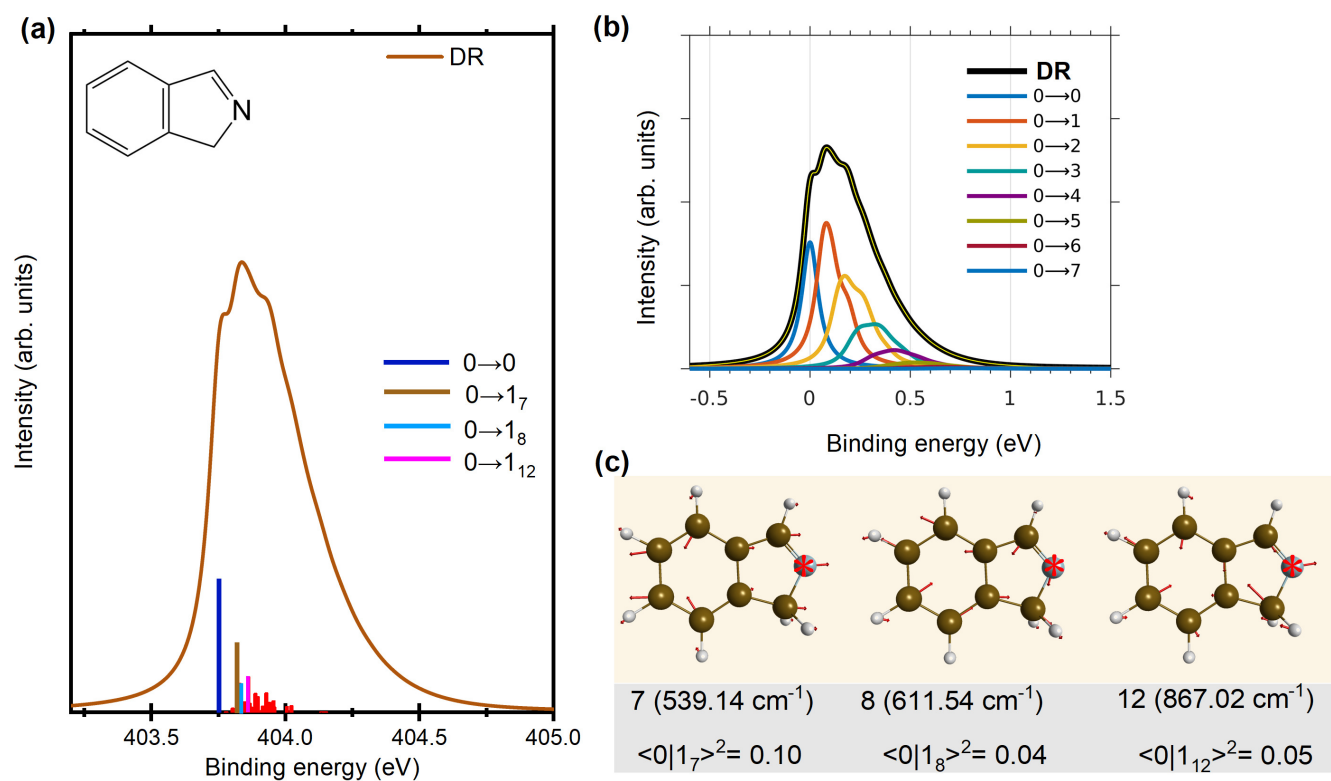

FIG. S11: The same as Fig. S1 for 1H-isoindole.

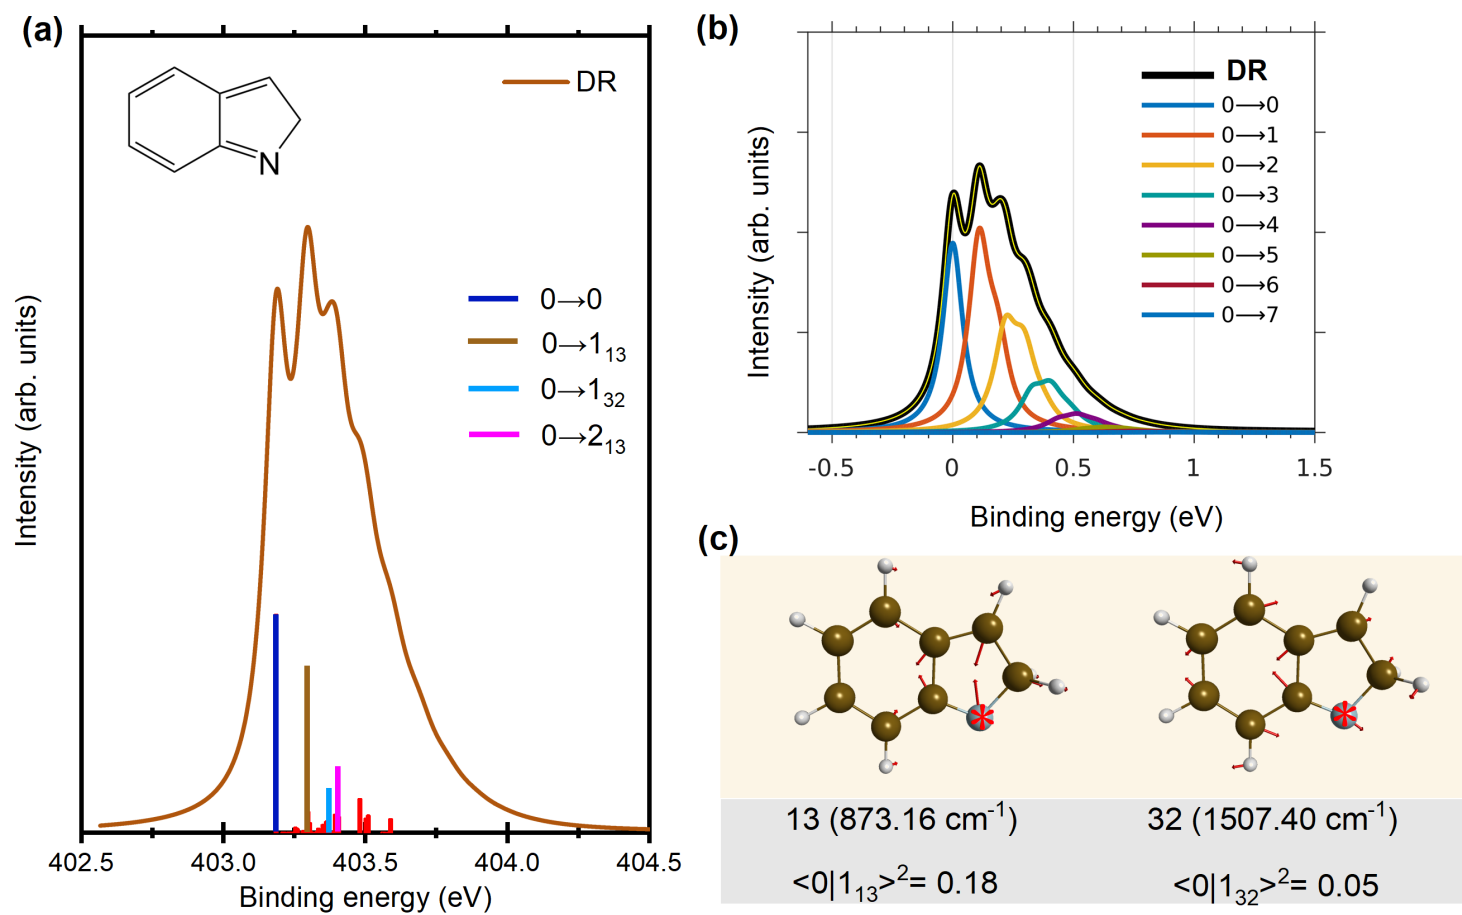

FIG. S12: The same as Fig. S1 for 2H-indole.

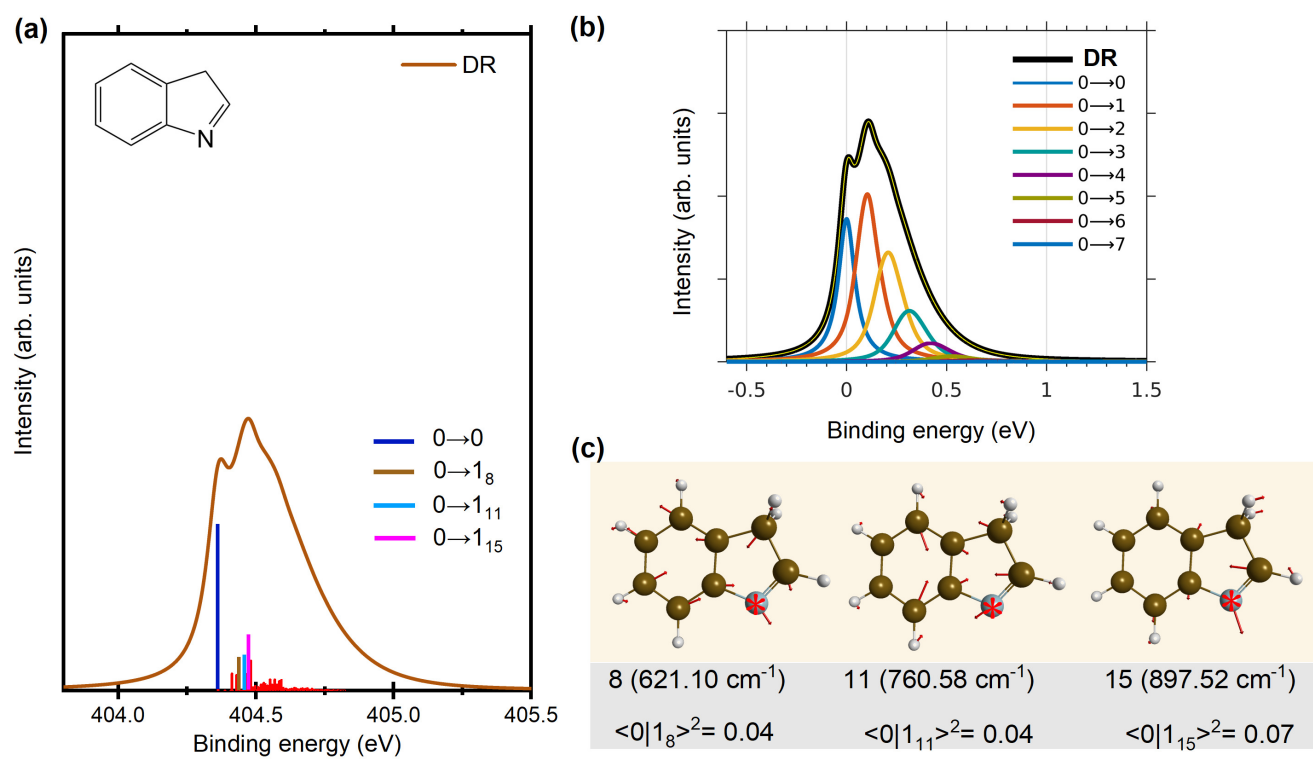

FIG. S13: The same as Fig. S1 for 3*H*-indole.

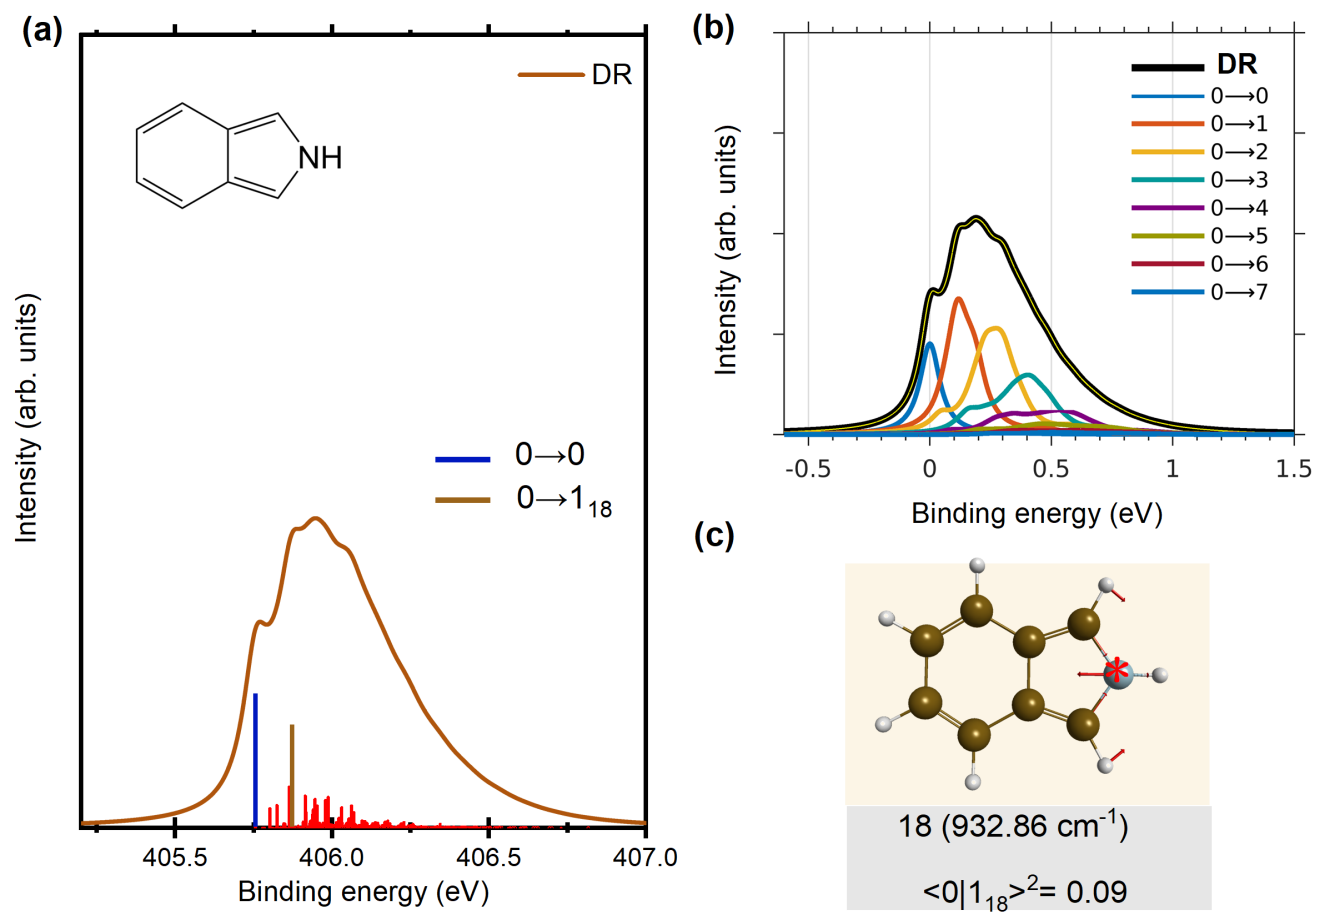

FIG. S14: The same as Fig. S1 for 2*H*-isoindole.

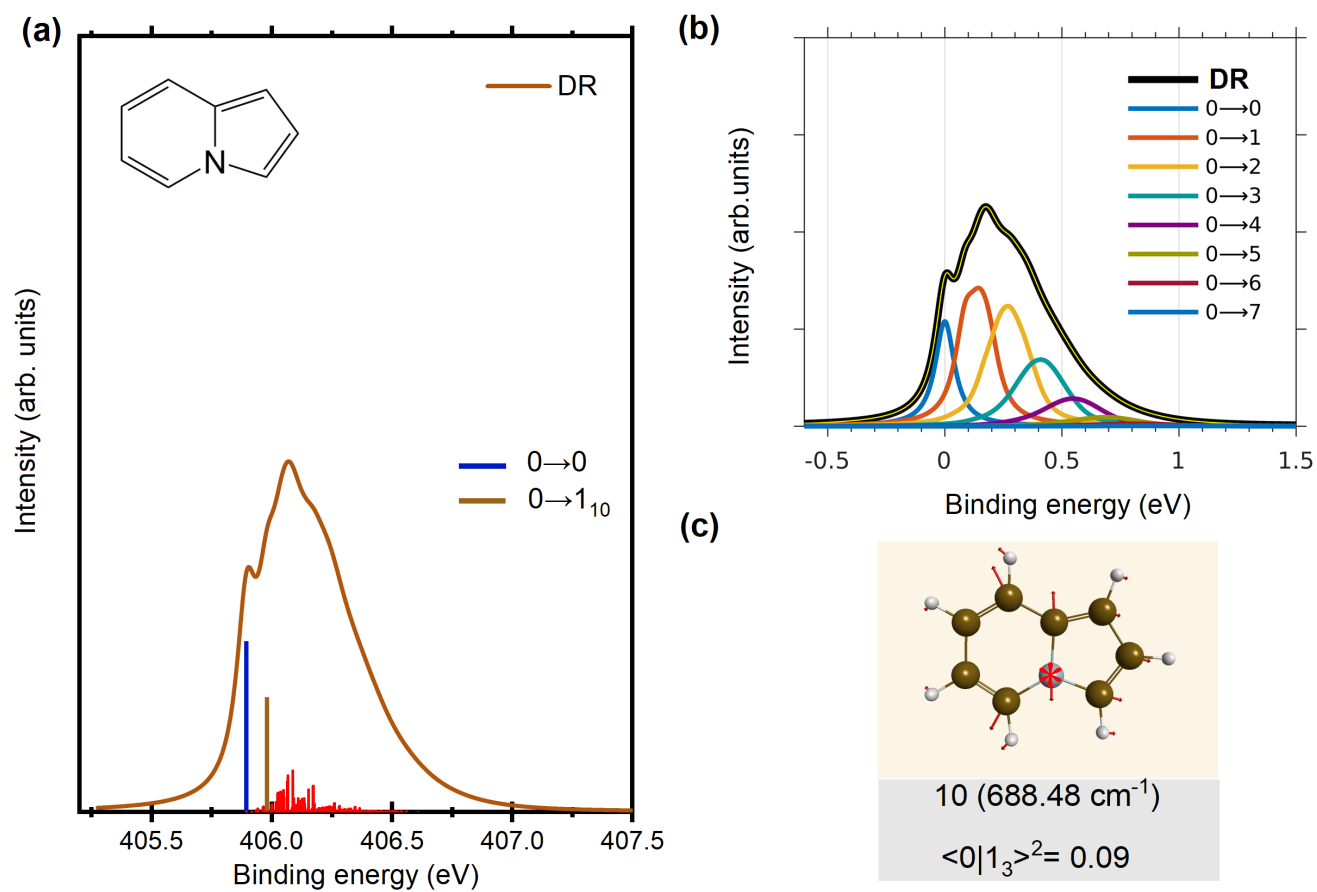

FIG. S15: The same as Fig. S1 for indolizine.

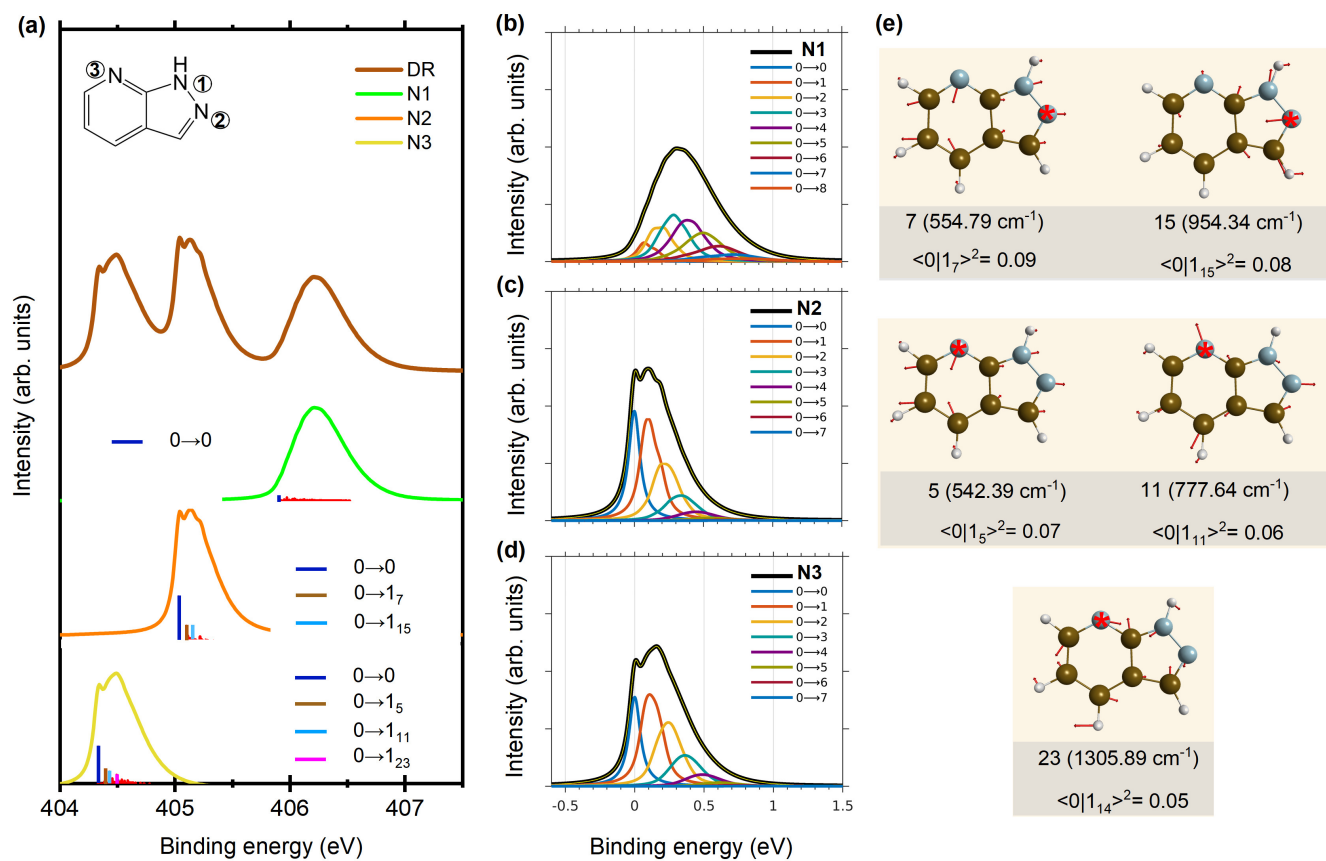

FIG. S16: (a) Simulated vibrationally-resolved N 1s XPS spectrum of 7-azaindazole. (b-d) The contribution of the different 0- $n$  transitions (until convergence) of N1-N3. 0-0 transition energy is taken as zero. (e) Active vibrational modes interpreted at the final state structure (**min FCH**). The core hole is indicated by an asterisk.

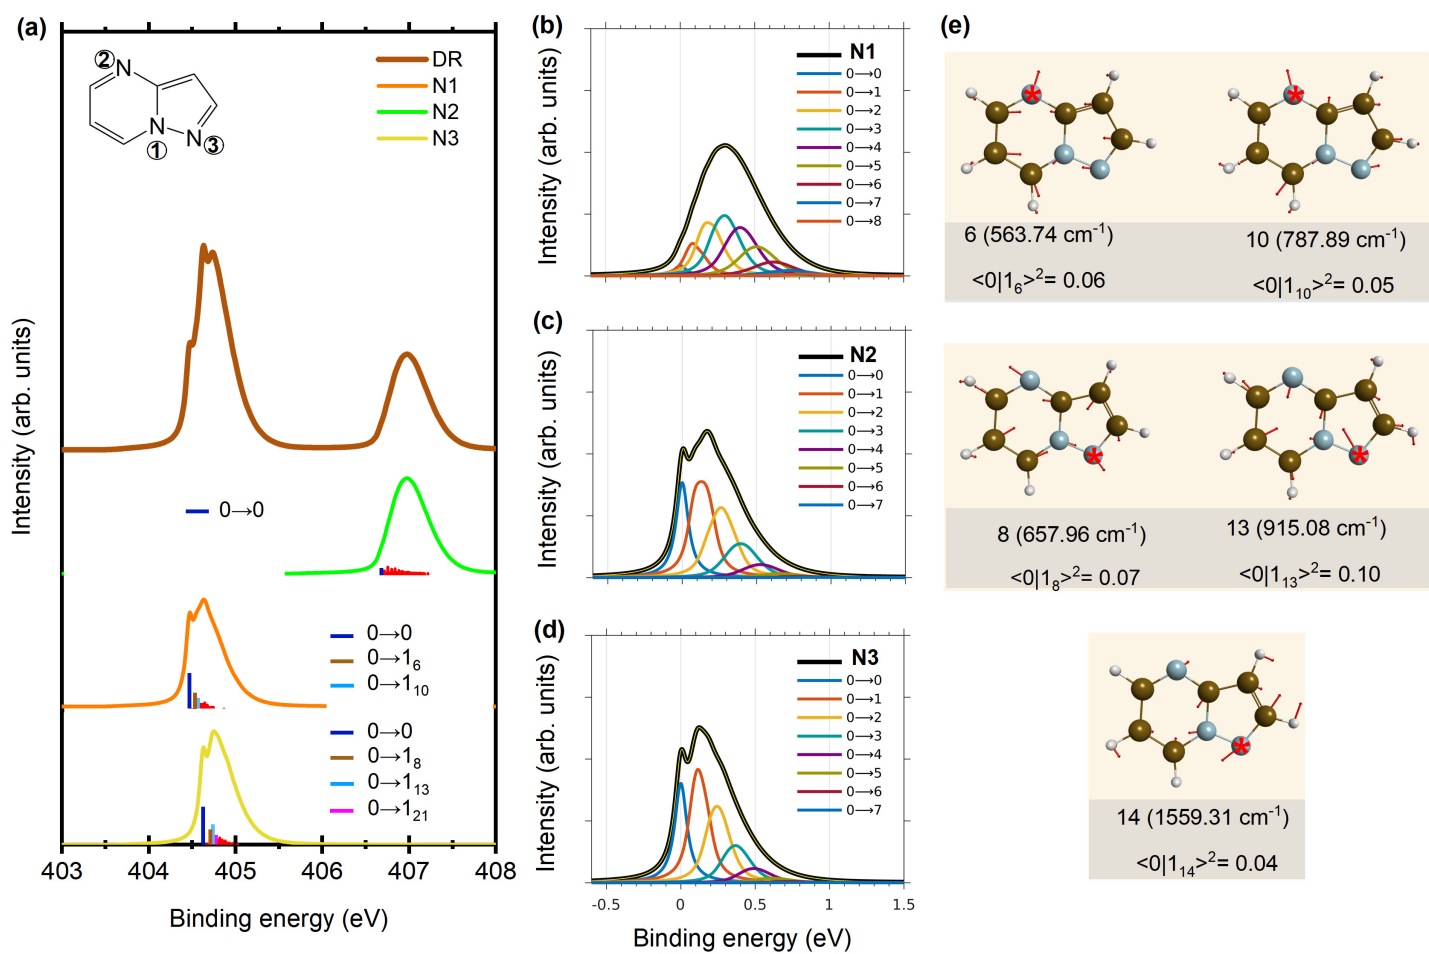

FIG. S17: The same as Fig. S16 for pyrazolo[1,5-a]pyrimidine.

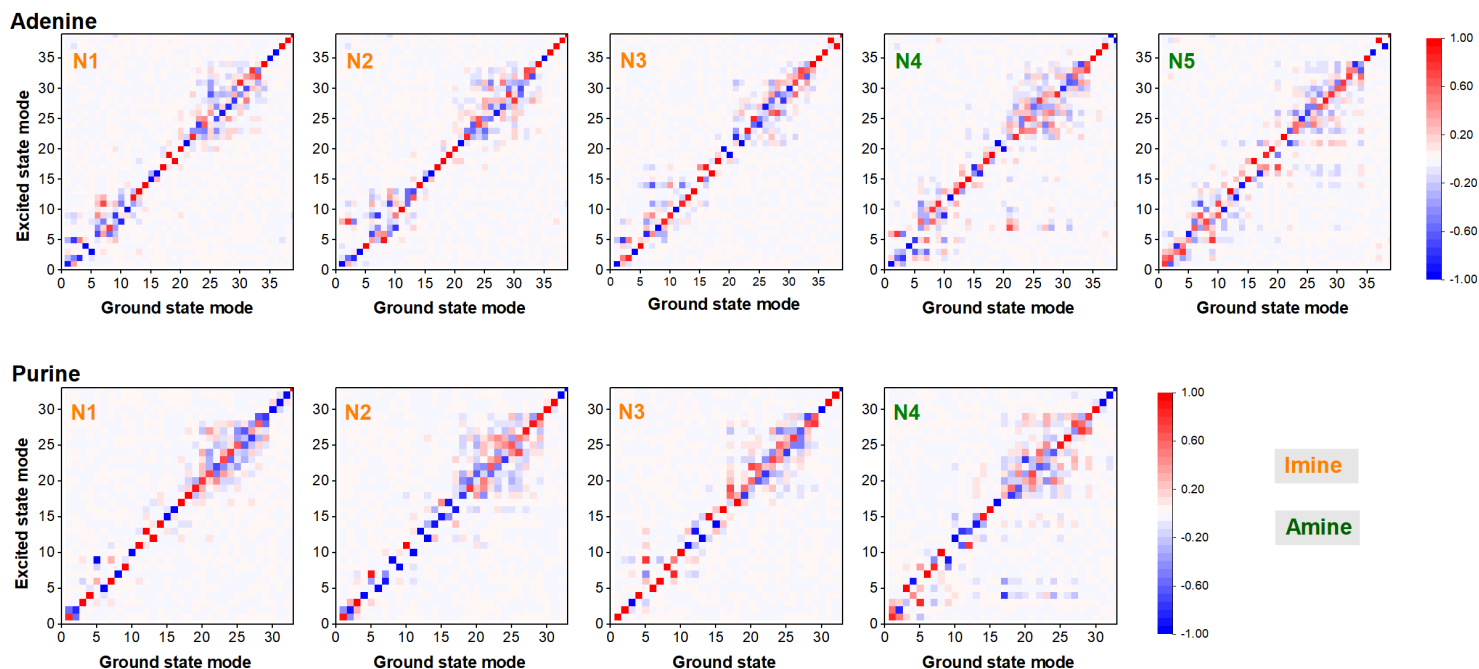

FIG. S18: Duschinsky matrices of purine and adenine. See structures and atomic labels in Fig. 1 of the main text. Amine (green) and imine (orange) N's are distinguished by colors.

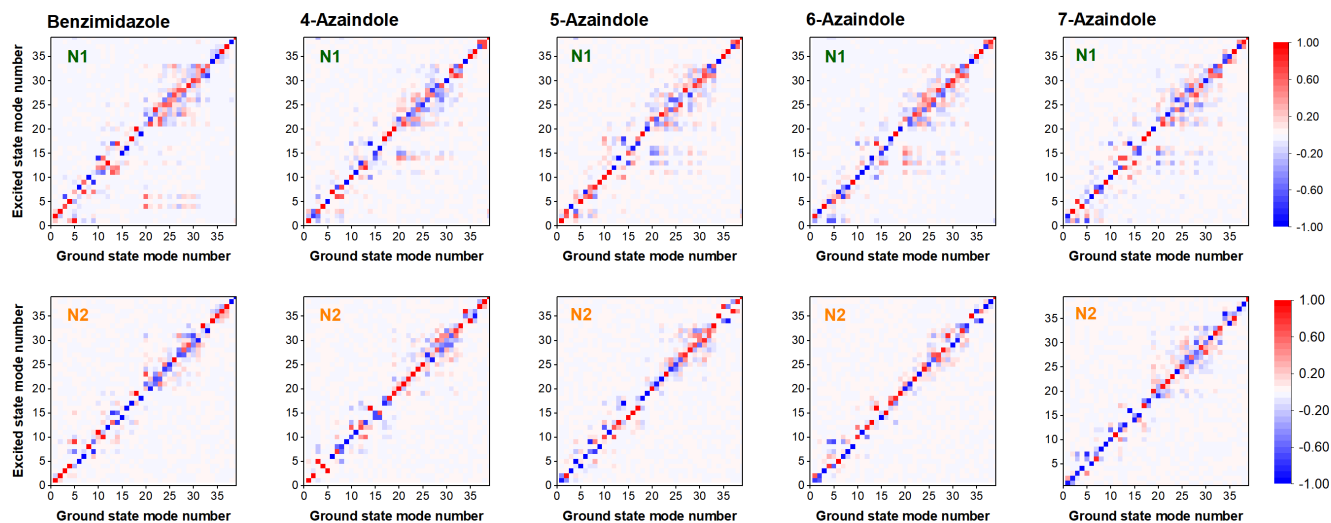

FIG. S19: Duschinsky matrices of benzimidazole, 4-azaindole, 5-azaindole, 6-azaindole, and 7-azaindole. See structures and atomic labels in Fig. 1 of the main text. Amine- (green) and imine- (orange) N's are distinguished by color.

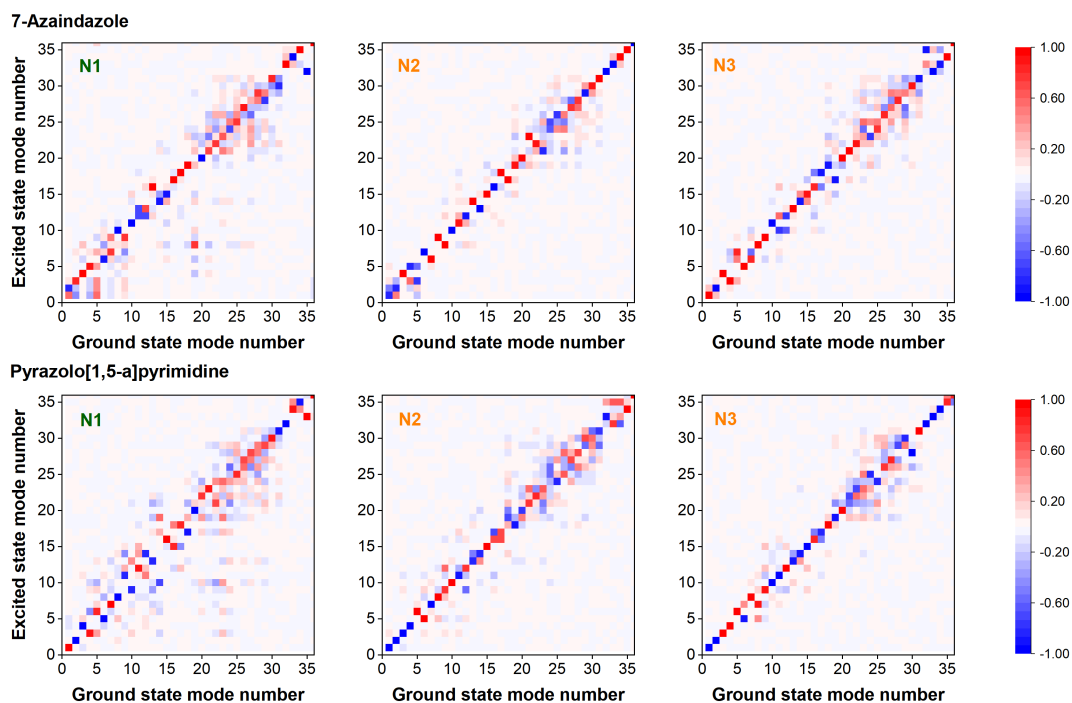

FIG. S20: Duschinsky matrices of the 7-azaindazole and pyrazolo[1,5-a]pyrimidine. See structures and atomic labels in Fig. 1 of the main text. Amine (green) and imine (orange) N's are distinguished by color.
